# Supplementary material for: Efficient Diffusion as Low Light Enhancer
Source: arXiv:2410.12346 source file (2026-03-18)
Supplement: Supplementary file 1 [file X_suppl.tex]

\clearpage
\setcounter{page}{1}
\maketitlesupplementary

\section{Proof of Corollary 1}
Given $ \tilde{x}_0 $, it can be represented into the noisy states according to the forward process of diffusion models as follows:
\begin{equation}
    \begin{aligned}
        \tilde{x}_0 = \frac{x_t - \sigma_t \tilde{\epsilon}}{\alpha_t},
    \end{aligned}
    \label{eq: tilde_x_0}
\end{equation}
Substitute \cref{eq: tilde_x_0} into $\tilde{x}_s = \alpha_s \tilde{x}_0 + \sigma_s\epsilon_\eta $, we get:
\begin{equation}
    \begin{aligned}
        \tilde{x}_s & = \alpha_s \tilde{x}_0 + \sigma_s\epsilon_\eta \\
        & = \frac{\alpha_s}{\alpha_t}x_t - \frac{\alpha_s}{\alpha_t}\sigma_t \tilde{\epsilon} + \sigma_s\epsilon_\eta(x_{u}, y, u),
    \end{aligned}
\end{equation}
Given the teacher trajectory $x^\eta_{s,u,t}$ defined in the main paper:
% \cref{eq: teacher_traj} ------------ Equation~(\textcolor{cvprblue}{4})
\begin{equation}
    \begin{aligned}
    x^\eta_{s,u,t} &= \frac{\alpha_s}{\alpha_t}x_t + \sigma_s\epsilon_\eta(x_{u}, y, u) \\ 
    &+ \frac{\alpha_s}{\alpha_u} \sigma_u (\epsilon_\eta(x_{t}, y, t) - \epsilon_\eta(x_{u}, y, u)) \\
      & - \frac{\alpha_s}{\alpha_t} \sigma_t\epsilon_\eta(x_{t}, y, t),
    \end{aligned}
\end{equation}
we can obtain the following equation:
\begin{equation}
    \begin{aligned}
    & \omega x^{\eta}_{s,u,t} + (1 - \omega) \tilde{x}_s \\
    & = \frac{\alpha_s}{\alpha_t}x_t + \sigma_s\epsilon_\eta(x_{u}, y, u)  \\
    &+ \omega  \frac{\alpha_s}{\alpha_u} \sigma_u \Big(\epsilon_\eta(x_{t}, y, t) - \epsilon_\eta(x_{u}, y, u)\Big) \\
      & - \frac{\alpha_s}{\alpha_t} \sigma_t \Big(\omega \epsilon_\eta(x_{t}, y, t) +  (1-\omega)\tilde{\epsilon}\Big) \\
      & = \tilde{x}^{\eta}_{s,u,t}.
    \end{aligned}
\end{equation}
 
\section{Implementation details}
We train our teacher models for 2 million iterations with the framwork of SR3 on the Gaussian flow \cite{SR3}. In the distillation stage. and 5000 iterations is required. We employ the Adam optimizer with a learning rate of $1 \times 10^{-4}$, applying linear weight decay. To stabilize training, we utilize an exponential moving average (EMA) with a weight of 0.9999 during parameter updates in both the pretrain and distillation stages. We adopt a fine-grained diffusion method with $T = 512$ steps and implement a linear noise schedule with endpoints set at $1 \times 10^{-4}$ and $2 \times 10^{-2}$. The patch size and batch size are set to 96 and 16, respectively. All the experiments are run on a single A100 GPU with 80GB of memory. Training our method with a smaller patch size and batch size on a device with less memory is feasible.

\section{Dataset}

\textbf{LOLv1} comprises 485 pairs of low/normal-light images for training and 15 pairs for testing, taken under different exposure conditions. \textbf{LOLv2} is divided into LOLv2-real and LOLv2-synthetic subsets. LOLv2-real contains 689 pairs for training and 100 for testing, adjusted for exposure time and ISO. LOLv2-Synthetic is created by analyzing the illumination distribution of low-light images, comprising 900 pairs for training and 100 for testing.

\noindent\textbf{SID.} The subset of the SID dataset captured by a Sony camera is adopted for evaluation. There are 2697 short-/long-exposure RAW image pairs. The low-/normal-light RGB images are obtained by using the same in-camera signal processing of SID \cite{sid} to transfer RAW to sRGB. 2099 and 598 image pairs are used for training and testing. \textbf{SDSD.} We adopt the static version of SDSD, captured by a Canon EOS 6D Mark II camera with an ND filter. We use 62:6 and 116:10 low-/normal-light video pairs for training and testing on indoor subsets.

\noindent\textbf{ DICM, LIME, MEF, NPE, and VV.} We evaluate the generalization capability of our models trained on the LOLv1 and LOLv2 datasets by testing them on the DICM, LIME, MEF, NPE, and VV datasets. Since these datasets lack ground truth images, evaluation relies on visual comparison and no-reference image quality assessment methods. 

\section{More experiment results} \label{sec:2}
\begin{figure}[t]

\centering
\includegraphics[width=0.95\linewidth]{./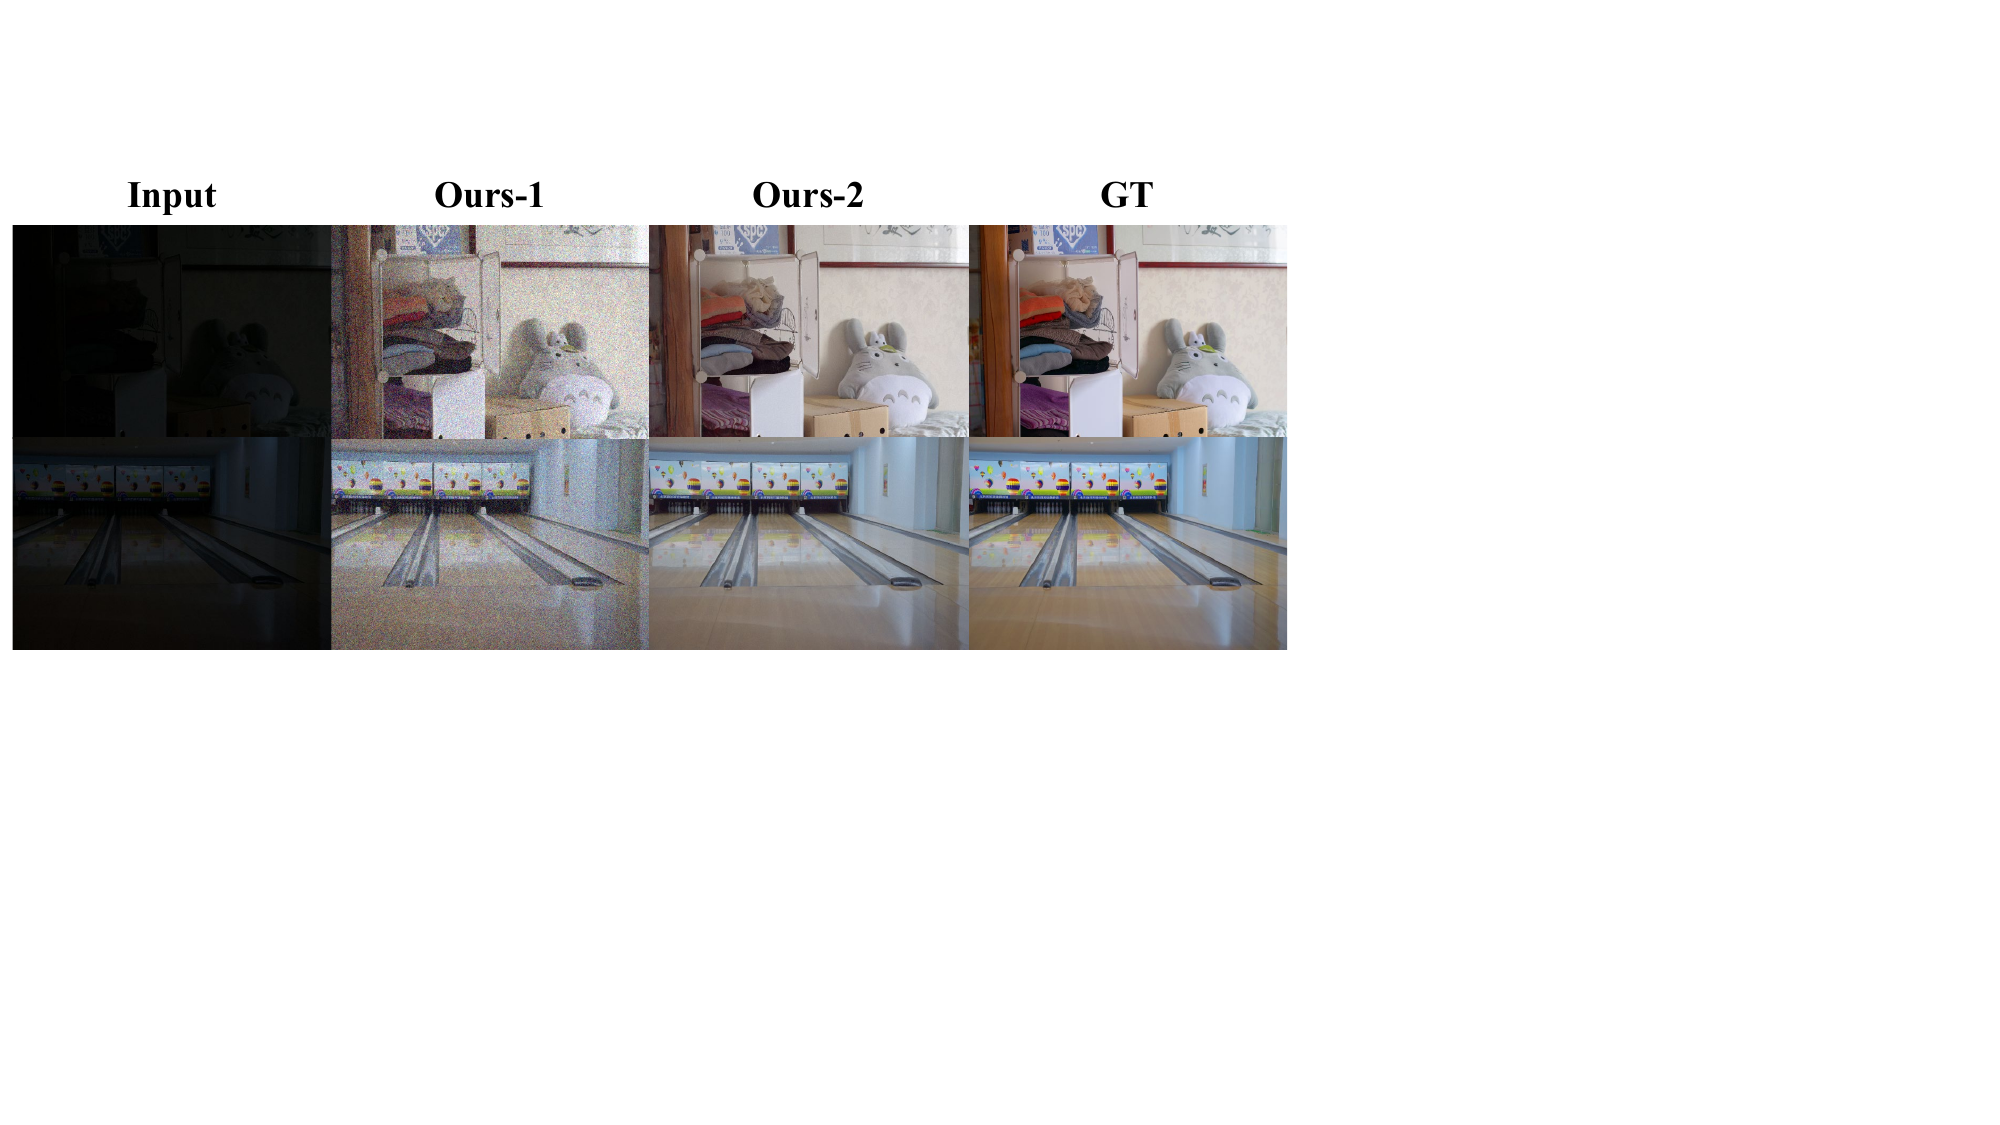} 

\caption{Failure cases in the single step.}
\vspace{-0.5cm}
\label{fig:failure_case}
\end{figure}
\subsection{The failure cases in one-step restoration.} 
As discussed in the limitation, ReDDiT struggles with single-step image restoration. Unlike single-step diffusion in image generation, which primarily introduces artifacts, single-step diffusion in LLIE mainly introduces noise. This brings a new insight into LLIE: the overall structure is constructed by the single-step diffusion, while iterative sampling enhances restoration results through denoising. The qualitative results of single-step restoration are demonstrated in \cref{fig:failure_case}.

\begin{figure*}[t]

\centering
\includegraphics[width=0.95\linewidth]{./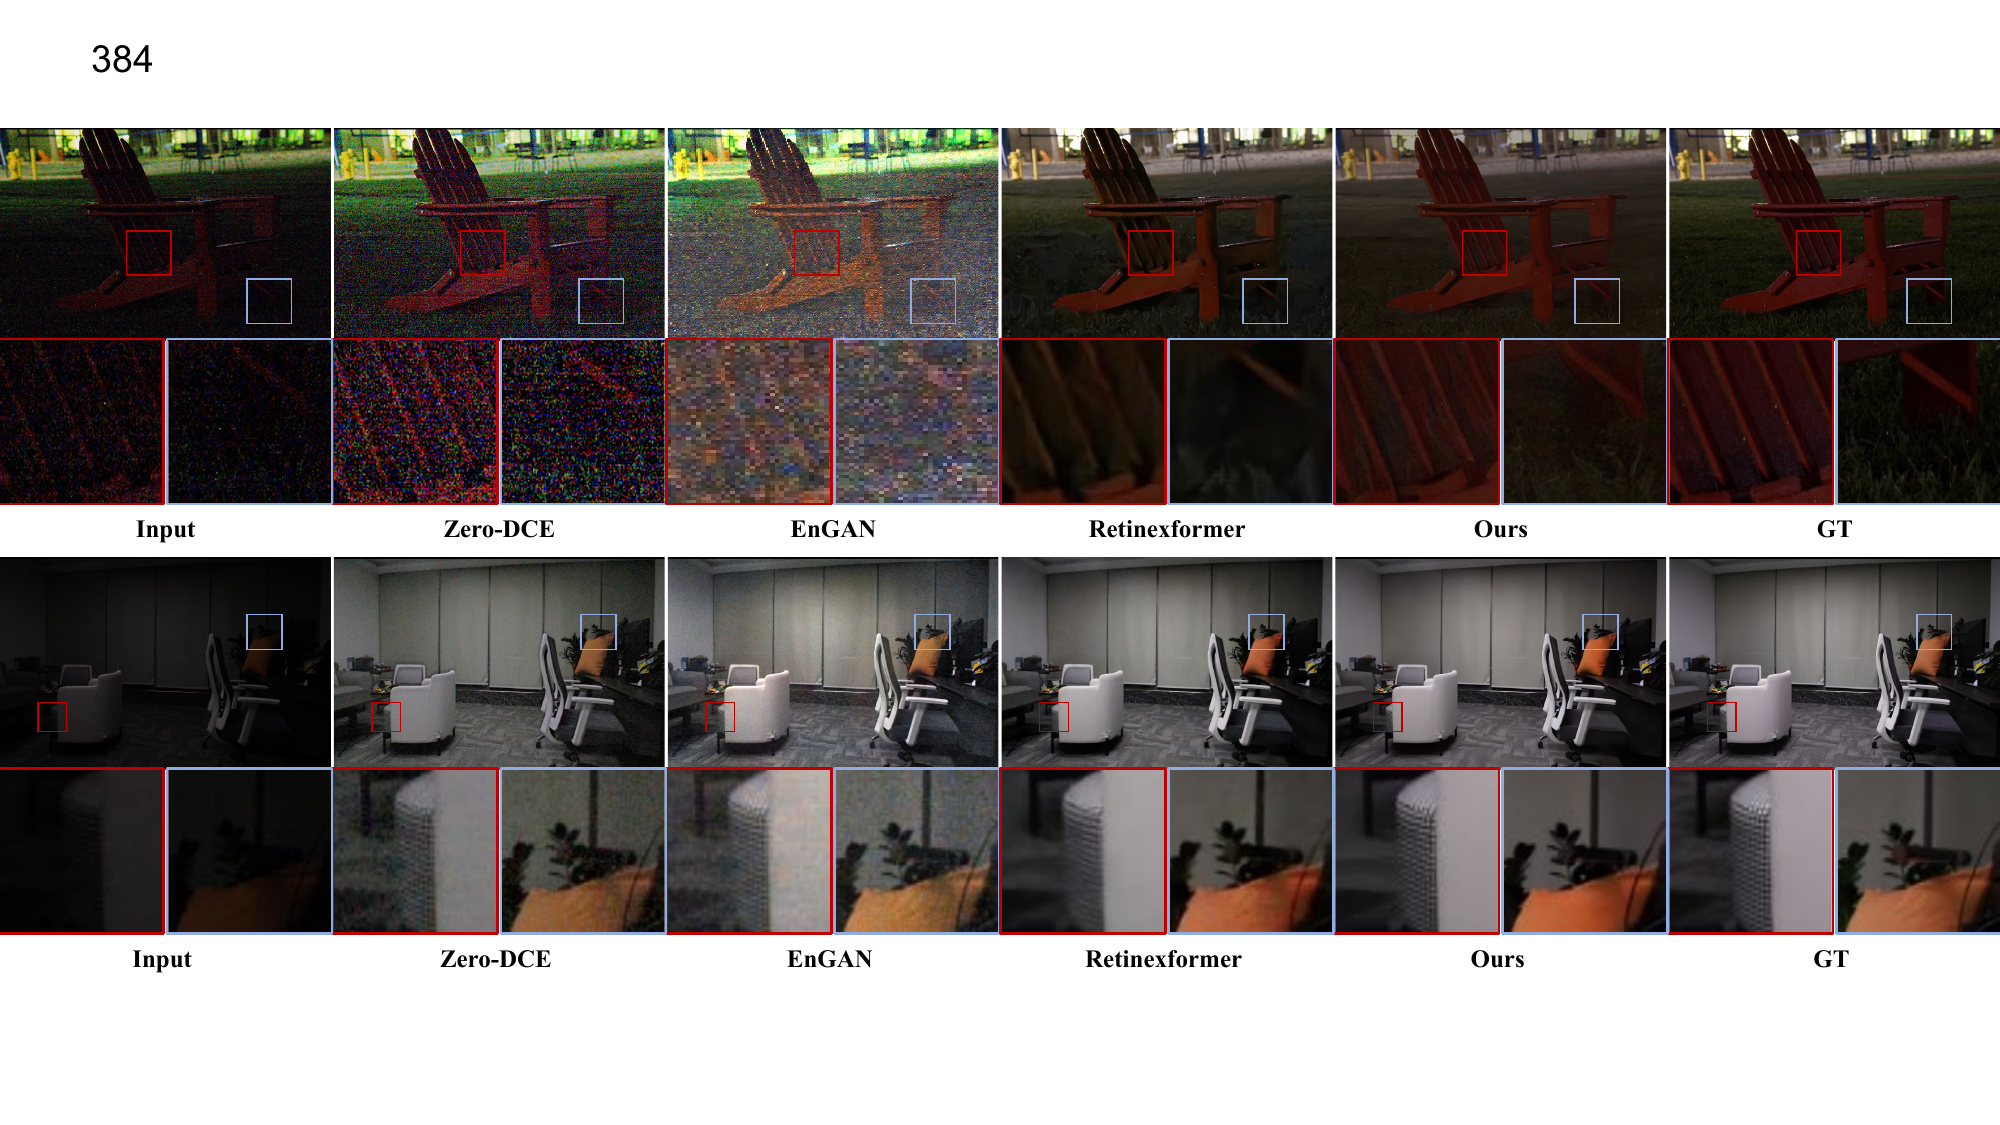} 
 \caption{Qualitative results on SID and SDSD. Patches highlighted in each image by the red and blue boxes indicate that ReDDiT \emph{effectively enhances the visibility, preserves the color, reduces noise, and retains finer details in normal light images}. It can be observed that the visual results of our method align more closely with the ground truth. Please zoom in for a clearer view of the image details.}
\label{fig:sid_sdsd}
\end{figure*}

\begin{figure*}[t]
\centering
\includegraphics[width=0.95\linewidth]{./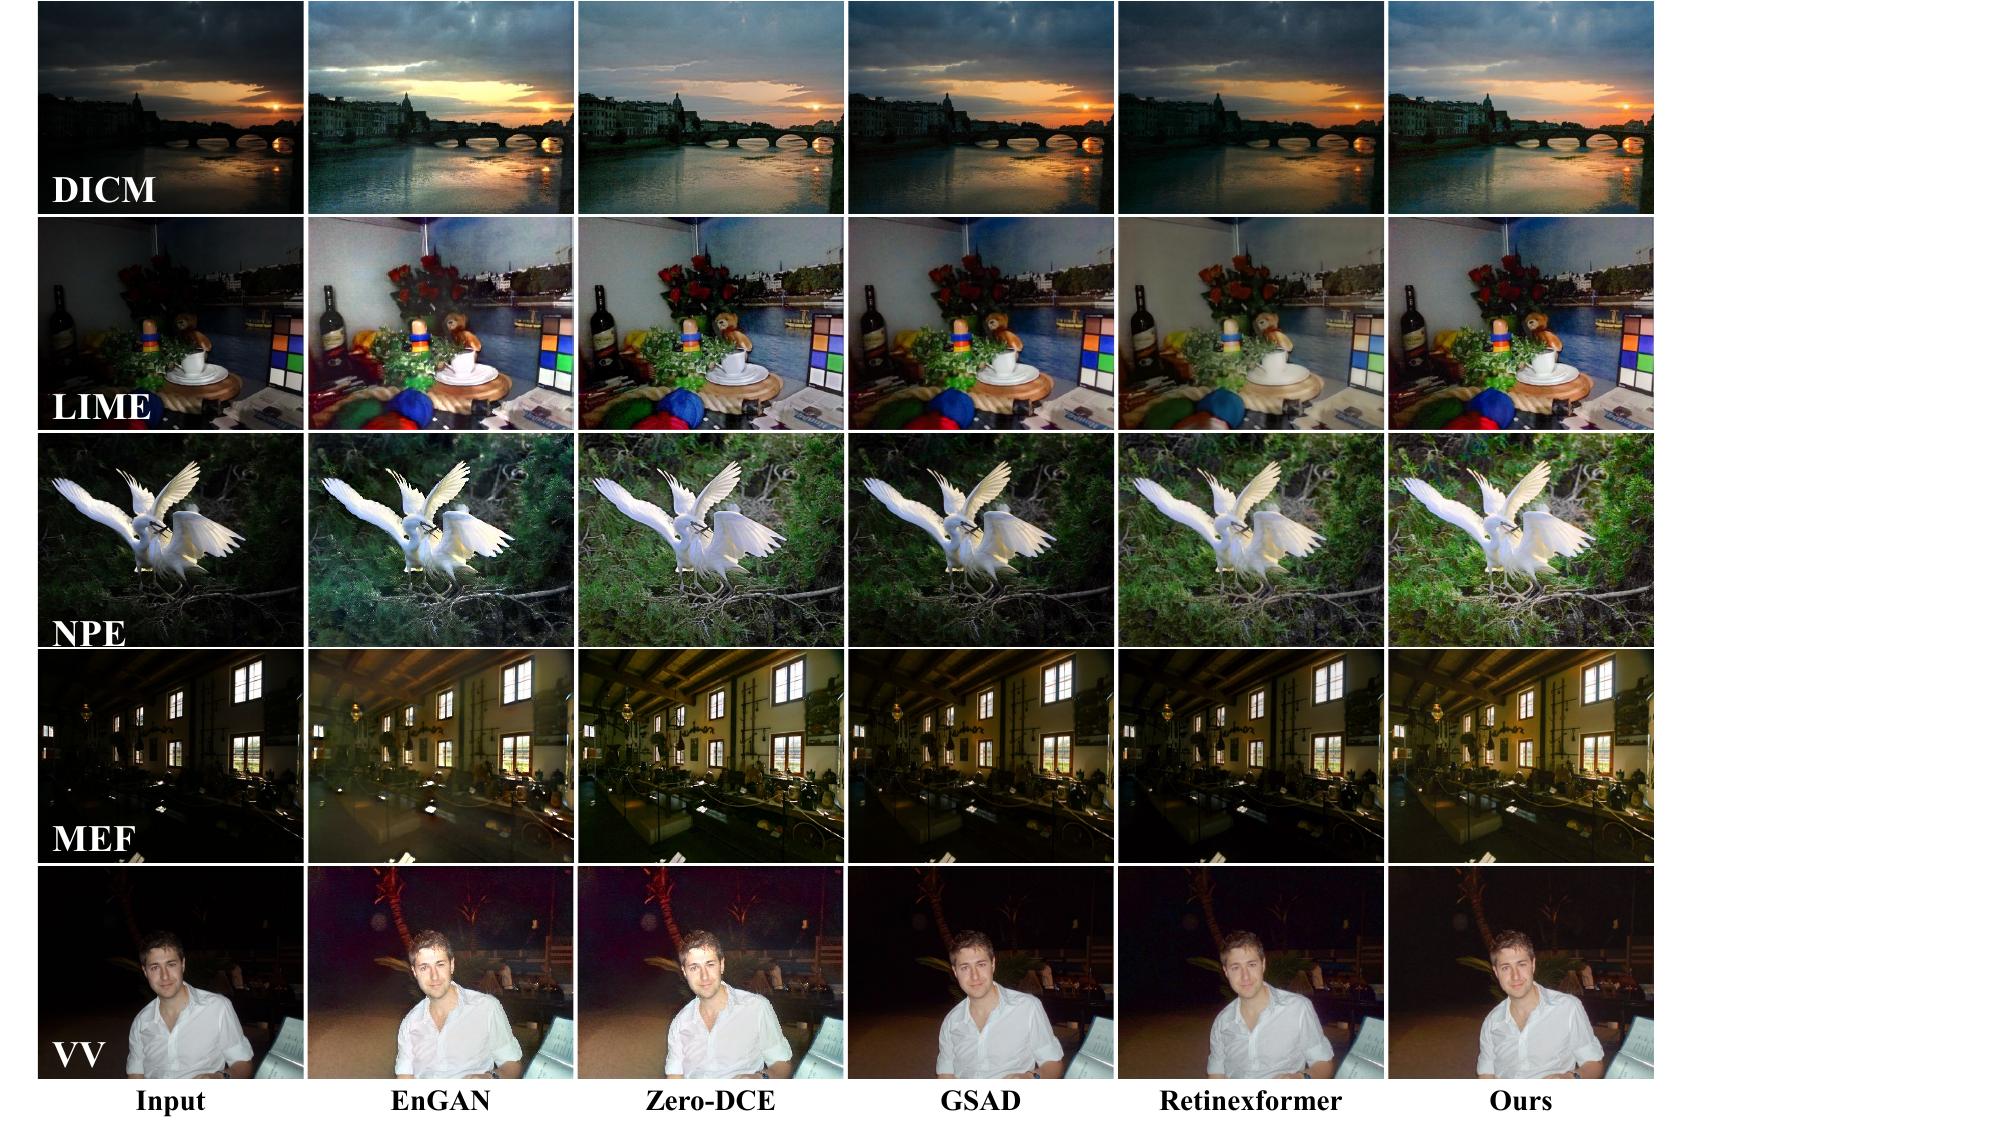} 
 \caption{Qualitative results on DICM, LIME, NPE, MEF, and, VV. Our method effectively enhances the visibility and preserves the color. Please zoom in for a clearer view of the image details.}
\label{fig:unpair_supp}
\end{figure*}

\subsection{Visual comparison on SID and SDSD dataset} 
Due to space constraints in the main manuscript, we only presented quantitative comparisons. Here, we offer additional visual comparisons on the SID \cite{sid} and SDSD \cite{sdsd} datasets in \cref{fig:sid_sdsd}. These datasets pose significant challenges for low-light image enhancement due to both low light levels and severe noise degradation. Our ReDDiT method demonstrates strong performance in improving brightness and reducing noise on these challenging datasets It can be observed in \cref{fig:sid_sdsd} that our ReDDiT \emph{effectively enhances the visibility, preserves the color, improves noise reduction, and retains finer details in normal light images}.

\subsection{Visual comparison on Unpair dataset} 
Due to space limitations in the main manuscript, we only provided visual comparisons with GSAD \cite{hou2024global}. In \cref{fig:unpair_supp}, we offer additional visual comparisons on DICM, LIME, NPE, MEF, and VV datasets. These results demonstrate the generalizability of ReDDiT to real-world low-light image enhancement scenarios and its consistent performance and superiority in preserving image details and improving visibility, making it a reliable solution for real-world applications.
